# Supplementary material for: Characterizing Grounded Theory Approaches in Visualization
Source: arXiv:2203.01777 source file (2022-04-21)
Supplement: Supplementary file 1 [file appendix-A.tex]

\section*{\textbf{A. Variables and Categories}}
\label{app:Categories}
%
This appendix contains the specification of the categorization scheme used in this paper. The part of the scheme for human coding was obtained after a number of iterative GT processes. Following the GT principles, the categorization scheme will continue to evolve until it reaches theoretical saturation.

\subsection*{A.1 Terminology and Criteria}
%
The following terminology is used in this work. 
%
\begin{itemize}
  \vspace{-1mm}
  \item \textbf{Variable} --- a variable defines a \emph{concept} (e.g., color) that may have different \emph{states} (red, yellow, green, etc). In a different context, it is often referred to as \emph{variable name} (when a variable is confusingly meant as a value), \emph{alphabet} (in information theory), \emph{dimension} (in dimensionality reduction), \emph{factor} (in factor analysis), \emph{parameter} (in system settings), \emph{column heading} (in spreadsheet), etc. The terms that may cause confusion and should not be used to mean a variable include class, attribute, value, etc.
  \vspace{-1mm}
  \item \textbf{Category} --- is a \emph{state} of a \emph{concept}. A concept can have an infinite number of states (e.g., an integer number). The term is usually used in conjunction with nominal or ordinal variables, which are also referred to as categorical variables. In general, a category is a \emph{valid value} of a variable. The adjective ``valid'' is necessary for a category (e.g., there are two different colors among five apples -- red and green), as a value can also mean an instance (e.g., five apples are of red, red, red, green, green). In a different context, a category or a valid value may be referred to as \emph{options} (in a set of radio buttons), \emph{letter} (information theory), etc. A variable can be defined with an infinite number of categories.
  \vspace{-1mm}
  \item \textbf{Categorization Scheme} --- A categorization scheme typically consists of $N$ \emph{variables} ($N > 0$), and each variable is defined with a set of categories. 
  \vspace{-1mm}
  \item \textbf{Categorization} --- This is a process for labelling a physical object or data object according to the variables and categories defined in a categorization scheme. The process is also referred to as classification.
  \vspace{-1mm}
  \item \textbf{Coding} --- In GT, the term \emph{coding} may imply categorization (e.g., selectively coding), defining categories through abstraction and grouping (e.g., open coding), comparing different optional categorization schemes (e.g., axial coding), or a combination of these in a single process. Its broad definition is likely related to the ambiguity of the word \emph{code}, which may mean a \emph{coding scheme} as well as a \emph{codeword} in a coding scheme.
\end{itemize}

The criteria for optimizing the specification of a categorization scheme (including its variables and categories) include:
%
\begin{itemize}
  \vspace{-1mm}
  \item The variables are reasonably orthogonal though it is almost impossible to assure their mutual independency.
  \vspace{-1mm}
  \item The categories in a variable must be mutually exclusive.
  \vspace{-1mm}
  \item When a post may feature elements that could potentially belong to different categories, we use word ``main'' in the definition of the variable, and word ``focus on'', ``mainly'', or ``at least'' etc. to define the boundaries between categories.
  \vspace{-1mm}
  \item The categories in a variable must cover all possible objects to be categorized (e.g., all posts).
  \vspace{-1mm}
  \item The boundary between categories should be easily determinable.
  \vspace{-1mm}
  \item Avoid a category “not applicable” as it is subjective to a 3rd party criterion for the reason ``why not applicable'', making this variable difficult to categorize independently.
  \vspace{-1mm}
  \item When a category relies on a human coder's subjective judgment that cannot be easily verified, the coder must write a commentary note.
\end{itemize}

\subsection*{A.2 Computer Coding per Post}
%
The VisGuides platform can provide each post with information according to the following variables as part of a categorization scheme automatically or algorithmically:

\begin{table}[h]
  \caption{Variables that can be coded by a computer.}
  \label{tab:Computer}
  \centering
  \begin{tabular}{@{}p{2.5cm}@{\hspace{2mm}}p{6cm}@{}}
    \toprule
    \textbf{Variables} & \textbf{Categories}\\
    \midrule
    \textbf{A1: Post ID} & Computer-generated ID numbers\\
    \textbf{A2: Topic} & (1) Cognition, (2) Education, (3) General, (4) Interaction,
                         (5) Medical Visualization, (6) Perception, (7) Site Feedback,
                         (8) Theory, (9) Uncategorized, (10) Visual Design, (11) VR/VE\\
    \textbf{A3: Thread} & Thread ID\\
    \textbf{A4: Thread Title} & Title of the thread or conversation\\
    \textbf{A5: Date} & Date\\
    \textbf{A6: Time} & Time\\
    \textbf{A7: Length-C} & The number of characters (letters, digits, etc.) in the post\\
    \textbf{A8: Length-W} & The number of words in the post\\
    \textbf{A9: Image} & The number of images included in the post\\
    \textbf{A10: TAR} & Thread-Author Relation: I or I1 (initiator), N (non-owner),
                        N2 (The 2nd person jointed thread), N3 (the 3rd person), ...\\
    \textbf{A11: TPR} & Thread-Post Relation: the ordered number of the posts within the thread,
                        1, 2, 3, 4, ...\\
    \bottomrule
  \end{tabular}
\end{table}

\input{sections/table-H1H2.tex}

\subsection*{A.3 Human Coding per Post}
%
After several iterations of open coding, axial coding, and selective coding, we have converged to six variables for the part of a categorization scheme to support human coding through close-reading. Although it may be possible in the future that some of such coding may potentially be done by a text analysis algorithm, we do not have any reliable algorithm for coding these variables yet. The involvement of humans in the coding process has brought about the most important scholarly benefit for defining the categorization scheme and understanding the relative merits of different ways of defining variables and categories.

During one iteration, we compared our categorization scheme with the Rhetorical Structure Theory (RST) by Mann and Thompson \cite{Mann:1988:TT} and the subsequent ontology by Mitrovi\'{c} et al. \cite{Mitrovic:2017:AC}. We also consulted the categorization scheme by Wachsmuth et al. \cite{Wachsmuth:2017:CL}, before our decisions on six variables, \textbf{H1. Main Purpose}, \textbf{H2. Guideline Mentioning}, \textbf{H3. Evidence}, \textbf{H4. Main Scope}, \textbf{H5. Antithesis}, and \textbf{H6. Conviction}, which are detailed in Tables \ref{tab:H1}-\ref{tab:H6}.

\input{sections/table-H3H4.tex}

\input{sections/table-H5H6.tex}


\subsection*{\textbf{A.4 Our GT Coding Process}}
%
Our methodology to code information from VisGuides followed the iterations of open coding, axial coding, and selective coding, together with memoing that records all the intermediate stages. 
As a result of applying GT, our coding scheme evolved in four main versions: $S_1$ to $S_4$. 
In this section, we use the following terminology:

\begin{itemize}[noitemsep,leftmargin=*]
    \item a \textbf{post} is an individual question or reply posted in the forum by a person. 
    \item A \textbf{thread} is an initial post plus the temporally-ordered sequence of all the replies, with the same ``(Thread) Topic'' in VisGuides. 
    \item A \textbf{question} is the post starting a thread. 
\end{itemize}


The coding was done mainly by two coders, $C_A$ and $C_B$, both of whom have been managing VisGuides and have read many of the posts before the coding started. Both coders, together with other team members have discussed possible research questions and hypotheses that one may be interested in grounding such questions on the data from VisGuides. Fig.~\ref{fig:GT-overview} shows the steps followed by the team in detail when applying GT.

To construct a categorization scheme, we followed the GT approach to ``orient'' potential variables towards our research questions. 
Example variables included \textit{`What are the questions asking for?'}, \textit{`How specific are the questions asking for advice?'}, and \textit{`Which guidelines are implicitly or explicitly mentioned in the threads'}. From this list of potential variables, we marked out all the information that would not require any human coding, such as \textit{number of replies per post}, \textit{posts per topic}, and dates. 
This left us with some candidate variables to consider in an iterative GT process involving open coding, axial coding, and selective coding.
There are many variables that could be used to characterize each post or thread, including but not limited to, those language variables for coding guideline statements used in \cite{kandogan2016grounded}; variables for coding visualization topics, users, tasks, and applications; and variables about the discourses where guidelines are discussed.
In our coding exercise, our data and our research questions directed us to focus on the variables that are featured in the data and can be used to answer our research questions. 

% In addition, to code guidelines, visualizations, and visualization topics mentioned (e.g., color perception, 3D visualization, user tasks, etc.). Note that the latter three are not \textit{categories} in the sense of GT, but required human coding. 


%Then, two of the paper authors started reading a random set of around 9 threads, trying to find find representative categories for each of our 10 dimensions to classify that thread. After coding these articles and discussing our coding, we established our first formal categorization scheme C1.

\begin{figure*}[t]
    \centering
    \includegraphics[width=140mm]{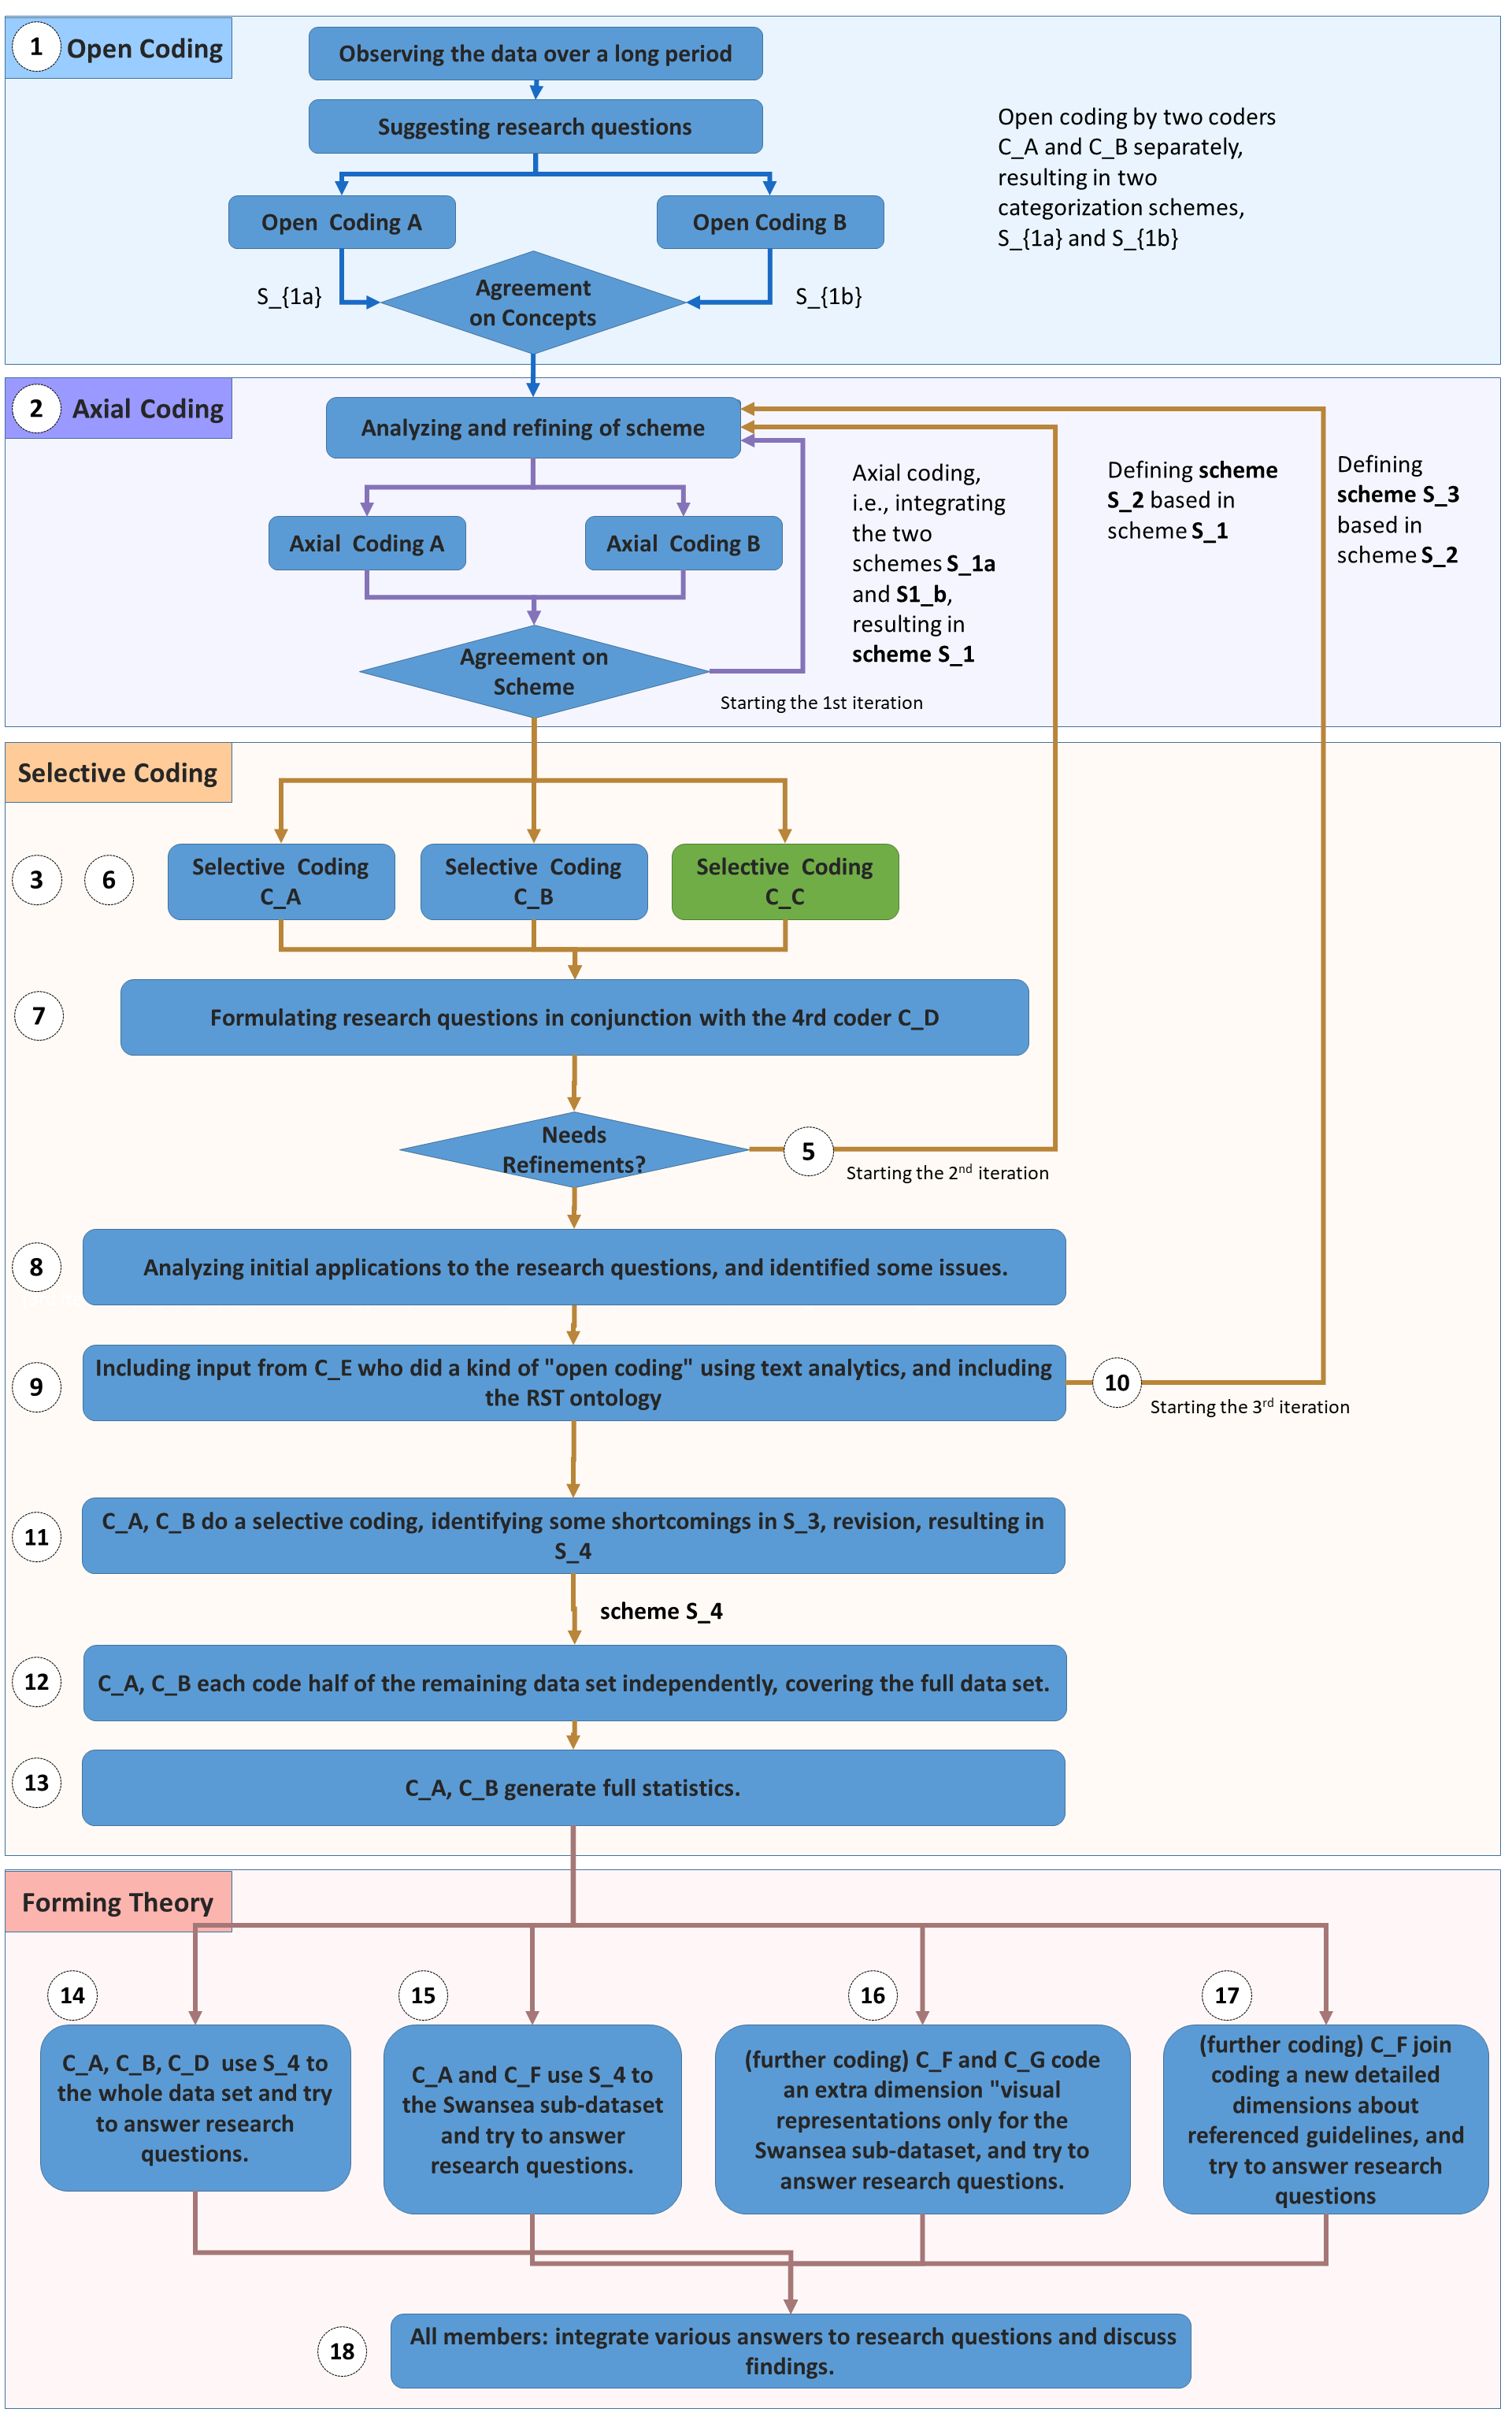}
    \caption{A task workflow chart showing the different steps of our GT coding process. The tasks are grouped in four main stages in GT: open coding, axial coding, selective coding, and theory formation~\cite{dillon2012grounded}.}
    \label{fig:GT-overview}
    % \vspace{-20mm}
\end{figure*}

\begin{enumerate}[noitemsep,leftmargin=*]
  \item \textbf{Starting the first iteration, aiming for $S_1$.} -- The two main coders, $C_A$ and $C_B$ first open-coded the data independently, resulting in two categorization schemes $S_{1a}$ and $S_{1b}$. For this iteration, both coders formulated their variables and categories on a per-\textit{thread} basis, i.e., considering all posts in each thread as a whole. 
  
  \item $C_A$ and $C_B$ then conducted axial coding, integrating the two independent categorization schemes. This resulted in scheme $S_1$, which contained 6 dimensions with 21 categories in total. Additionally, we defined some plain-text categories, characterizing how the discussions in a thread was evolving (e.g., ``single-reply'', ``first reply says the given guideline is too strict, then points to literature for general advice'', etc.), and which guidelines and which topics were mentioned.
  
  \item $C_A$ and $C_B$, with the help of a third coder $C_C$ (an MSc student), then applied $S_1$ to a subset of the data, i.e., selective coding the 10 threads with the most replies. 
  
  \item All three coders $C_A$, $C_B$, $C_C$ then discussed the scheme $S_1$ and the coding results. During the discussion, $C_A$ and $C_B$ agreed that coding on a per-thread basis was too coarse to establish a suitable categorization scheme since threads contained too much and too rich information and thus required the coders to make too many complex decisions.

  \item \textbf{Staring the second iteration, aiming for $S_2$.} -- This time, we aimed for coding on a paragraph-basis, i.e., coding individual paragraphs in each post. Based on the discussion about $S_1$, $C_A$ and $C_B$ refined the dimensions to obtain an $S_2$, which included 5 dimensions (\textit{How is the guideline expressed?} \textit{How suggestive is the statement?}, \textit{Is the statement mentioning any conditions?}, \textit{How is the statement supported?}, and \textit{How generalizable are the statements to other topics in visualization?}). These dimensions included 27 categories in total.

    %\item $C_A$ and $C_B$ then, again open-coded independently bases on $S_2$, resulting in $S_{2a}$ and $S_{2b}$.
 %\item $C_A$ and $C_B$ then, again conducted open-coding independently, oriented towards the research questions, resulting in two categorization schemes,$S_{2a}$ and $S_{2b}$.
  \item $C_A$ and $C_B$ conducted selective coding independently by applying $S_2$ to a subset of the data. When analyzing the coding results, $C_A$ and $C_B$ found a fair amount of disagreement in the coding results. The coding on a per-paragraph basis again turned out to require too many complex decisions from the coders, including the decision on how to split the posts into meaningful units. Moreover, we found that many paragraphs contain similar information and hence would have preferred to combine them into a higher level unit. In summary, we found coding on a per-paragraph basis too fine-grained. That was an obstacle to continue with the next step, i.e., applying $S_2$ to the whole data set, and we anticipated that the results would not provide adequate support to the stage of ``Forming Theories''. We decided that the best way forward was to code on a per-post basis.
  
    %In particular, we found coding on a thread level too coarse to establish a clean coding since threads contained too much and rich information. 
  %Therefore, we decided to split the threads into posts, creating two data spaces: $D_{20190313}_1$ and $D_{20190313}_2$.
  
  %\item $C_A$ and $C_B$ selectively coded a number of examples using scheme $S_2$, with the help of an MSc student $C_C$.
%    These efforts resulted in a high degree of granularity and dispersion obstructing the extraction and construction of high level concepts and interrelations among the dimensions. That was an obstacle to continue with the next step of the methodology, ``Forming Theories'', so we decided to work with only one data space $D_{20190313}$, the data space of ``posts'' in VisGuides.
  
  \item $C_A$ and $C_B$, in conjunction with another researcher $C_D$, formulated research questions \textbf{Q1-Q3} as described in Section~\ref{sec:Introduction}. With the addition of $C_D$, we had established a more focused set of research questions and hypotheses that could be suitably grounded in our data. We discovered several challenges related to the completeness and independence of the existing variables.
  
  \item $C_A$ and $C_B$ revised $S_2$, resulting in $S_2'$, in order to make it work with posts, and make it complete, errors free, and independent.
  $C_A$ and $C_B$ conducted another round of selective coding by applying $S_2'$ to the selected subset of the data, and analyzed the coding results to see if they could help answer the research questions, \textbf{Q1-Q3}. $C_A$ and $C_B$ saw the improvement of the new scheme $S_2'$ but also identified some further issues.
  
  \item $C_A$ and $C_B$ received some input from a team member, $C_E$, who had been observing the data using text analytics. As text analysis and visualization can be considered as open coding by the computer, the inputs were informative. $C_E$ also drew attention to the references of Rhetorical Structure Theory (RST).
 
  \item \textbf{Starting the third iteration, aiming for $S_3$.} --
  $C_A$, $C_B$, and $C_D$ conducted axial coding by integrating $S_2$ with some concepts in RST, resulting in scheme $S_3$. $S_3$ that focused on posts as an objective middle-granularity between paragraphs and threads.
   
  \item $C_A$ and $C_B$ selectively coded some data (i.e., the posts in the 10 threads with the most replies), and identified some shortcomings in $S_3$, and a revision resulted in the current categorization scheme $S_4$ discussed in Section \ref{sec:VisGuides} and detailed in Appendix A.3). We agreed on $S_4$ for the categorziation scheme for coding all posts in the data set $D_{20190313}$.
  
  \item $C_A$ and $C_B$ applied $S_4$ to code the full data set, by splitting the remaining data set into two equally sized parts and coding each part independently. 
  
  \item $C_A$ and $C_B$ generated some statistics on the frequency of categories to aid the examination of \textbf{Q1}, shown in Fig~\ref{fig:catstats}. The statistics based on human coding results allowed us to have a first glimpse into the summary overview visualization (as shown in Fig.~\ref{fig:catstats}), confirming some of the patterns that we have already observed during coding.
  
  \item $C_A$, $C_B$, and $C_D$ applied $S_4$ to answer research questions \textbf{Q1-Q2}, and used the computer-coded results to answer research question \textbf{Q3}.

  \item $C_A$ and another team member $C_F$ applied $S_4$ to the Swansea sub-dataset $D_{\text{Swansea2019}}$ and tried to answer research questions \textbf{Q4-Q5} related to the learning activities of Swansea students using their posts at VisGuides.
  
  \item \textbf{Additional Coding.} -- $C_F$ and $C_G$ coded an extra variable of ``visual representations'' for the Swansea sub-dataset to help answer research questions \textbf{Q4-Q5}.
  
  \item \textbf{Additional Coding.} -- another team member $C_H$ joined the coding effort for a new detailed variable about directly- and indirectly-referenced guidelines. This was to help answer research question \textbf{Q2} and the results are reported in Appendix B.
  
  \item We worked collaboratively to integrate the various answers to the research questions posed in the paper. The application of GT allowed us to examine the use of guidelines in different contexts, and identify several findings.
\end{enumerate}

\clearpage

% \textcolor{red}{Ben's old text below.}
% Our methodology to code information from VisGuides followed four major iterative open coding cycles, resulting in three classification schemes C1 to C3. Precise definitions for our final scheme can be found in the Appendix. In the following we use the terminology as follows: a \textit{post} is an individual question or reply posted in the forum by a person. A \textit{thread} is an initial post plus the sequence of replies. A \textit{question} is the post starting a thread. 

% First, to prepare a categorization scheme, we defined some dimensions based on our research questions that we would code for each thread.
% Example dimensions included \textit{`What are questions asking for?'}, \textit{`How specific are questions asking for advice?'}, and \textit{`Which guidelines are mentioned in the threads'}. From this scheme we marked all the information that would not require any human coding, such as \textit{number of replies per post}, \textit{posts per topic}, etc. This left us with 10 dimensions plus 3 dimensions capturing the guideline, the visualization, and the visualization topic mentioned in a reply. Note that the latter 3 are not \textit{categories} in the sense of GT, but were part of our human coding. Then, two of the paper authors started reading a random set of around 9 threads, trying to find find representative categories for each of our 10 dimensions to classify that thread. After coding these articles and discussing our coding, we established our first formal categorization scheme C1.

% \textbf{C1}---For this scheme we agreed 6 dimensions with 21 categories in total. Additionally, we coded how the discussion was evolving, which guidelines and which topics were mentioned. Two of the authors independently coded the 10 articles with the most replies. Upon discussion we found still large disagreement among the coding. In particular, we found coding on a thread level too coarse to establish a clean coding since threads contained too much and rich information. 

% \textbf{C2}---For C2, we decided to code \textit{by paragraph} of posts, rather than by \textit{thread}. We defined 5 dimensions (\textit{How is the guideline expressed?} \textit{How suggestive is the statement?}, \textit{Is the statement mentioning any conditions?}, \textit{How is the statement supported?}, and \textit{How generalizable are the statements to other topics in visualization?}). These dimensions included 27 categories in total. This time, the two of the coders, again individually, went over the 10 threads with most replies and split up the posts into paragraph whenever necessary. Upon discussion, we found the categories to work for most paragraphs. However, categorizing paragraphs turned out to be too fine grained and involve too much discussion about where to split if a paragraph contained several statements. 

%\textbf{C3}---For our final coding scheme, we decided to code \textit{posts} without splitting them into paragraphs. This final schema is explained below and can be found in the appendix for full reference. Including discussions with one more co-author, that scheme contains 6 dimensions with 30 categories in total. Since we focused on posts rather than paragraph, we coded according to the main purpose, evidence, tone, etc. of each post. Two coders independently coded the 20 articles with the most replies and the consequent discussion yielded very high agreement. We refined our category definitions one more time, to clarify the cases we disagreed in our coding. The two coders than each coded half of the remainder of of the 217 posts.



  
