# Supplementary material for: Characterizing Grounded Theory Approaches in Visualization
Source: arXiv:2203.01777 source file (2022-04-21)
Supplement: Supplementary file 2 [file appendix-B.tex]

\section*{\textbf{B. Mentioned Visualization Guidelines}}
\label{app:Guidelines}

This section lists all guidelines that are directly and indirectly mentioned in the posts between September 27, 2017 and March 13, 2019.

\subsection*{\textbf{B.1 Directly Mentioned Visualization Guidelines}}
\label{app:Direct}

The following guidelines have been directly mentioned in the discourses at VisGuides, and they are listed in the alphabetic order of the first keyword highlighted in bold. For guidelines with the same first keyword, the ordering is based on the second keyword, and so forth.   

\begin{itemize}[noitemsep,leftmargin=*]
  \item Do not use the \textbf{blow apart effects}. \cite{Duke:2019:web}
  
  \item The \textbf{Correspondence} Principle---The same data should produce the same visualization~\cite{Kindlmann:2014:TVCG}.
  
  \item Good visualization should maximize the \textbf{data-ink ratio}~\cite{tufte2001visual}.
  
  \item Facilitate \textbf{depth perception} for \textbf{3D} visualizations~\cite{borgo2013glyph}.
  
  \item \textbf{Feature-driven animation} vs. \textbf{interactive systems}:``Start with an overview of entire duration. End with a focused view in relevant time duration. Include all relevant data attributes in at least one segment of the animation sequence~\cite{Yu:2017:EI}.
  
  \item Shneiderman's  Visual \textbf{Information-Seeking Mantra}: Overview first, zoom and filter, details on demand~\cite{Shneiderman:1996:VL}.
  
  \item Use \textbf{interaction} in visualization sparsely and cautiously~ \cite{Groller:2008:Dagstuhl}.
  
  \item \textbf{Lie factor} guideline~\cite{tufte2001visual}: The representation of numbers, as physically measured on the surface of the graphic itself, should be directly proportional to the quantities represented.
  
  \item Don't use \textbf{more than six colors together}~\cite{Sayers:2019:web}.
  
  \item The \textbf{rainbow color} map is considered harmful~\cite{Rogowitz:1998:S,Borland:2007}

  \item \textbf{Reduce clutter} in parallel coordinates by reordering axes~\cite{Makwana:2016:IJCSIT}. 

  \item Elmqvist's Rule \#7: Don't \textbf{replicate} the \textbf{real world}~\cite{Elmqvist:2017:blog}.

  \item Few's Rule \#9: Avoid using \textbf{visual effects} in \textbf{graphs}~\cite{Few:2008:web}.
 
 \item \textbf{Visual variables} for visualizations in \textbf{VR}~\cite{Mackinlay:1986:TOG}
\end{itemize}

\subsection*{\textbf{B.2 Indirectly Mentioned Visualization Guidelines}}
\label{app:Indirect}

The following references to books, research papers, blogs, video, etc. have been been mentioned in the discussions on various topics, but there was no guideline mentioned explicitly in relation to these references. We consider that it is highly likely that most of these references contain some visualization guidelines. The references are listed according to firstly the topic categories and then the threads where the corresponding posts appeared. The topic categories are ordered alphabetically, and the thread headings are ordered alphabetically according to its keywords.

\paragraph{\textbf{Perception}}
\begin{itemize}[noitemsep]
    % \vspace{-1mm}
    \item The \textbf{rainbow color} map is considered harmful~\cite{MPL:2015:web, Rhyne:2016:book}.
\end{itemize}

\paragraph{\textbf{Theory}}
\begin{itemize}[noitemsep]
%   \vspace{-1mm}
  \item \textbf{Data-Ink Ratio} Principle, How to use it?~\cite{Strunk:2009:book,Behrisch:2019:CGF}.
\end{itemize}

\paragraph{\textbf{Visual Design}}
\begin{itemize}[noitemsep]
  \item \textbf{Clutter reduction} technique in \textbf{parallel coordinates}: \cite{Heinrich:2013:STAR}.
  \item Visual \textbf{Information-Seeking Mantra}: \cite{vanHam:2009:TVCG,Chen:2016:book,Luciani:2019:TVCG}.
  \item \textbf{Lie factor} guideline: \cite{Meihoefer:1973:Cartographica, Cleveland:1984:JASA}.
  \item Elmqvist's Rule \#7: Don't \textbf{replicate} the \textbf{real world}: \cite{Bach:2018:TVCG, Besancon:2017:CHI}.
  \item \textbf{Visual variables} for visualizations in \textbf{VR}: \cite{Chen:2014:BookChapter}
%   \vspace{-1mm}
  \item \textbf{Visualizing time} on a \textbf{geospatial map}: \cite{Weber:2001:InfoVis, VanWijk:1999:InfoVis} 
\end{itemize}
