# Supplementary material for: Characterizing Grounded Theory Approaches in Visualization
Source: arXiv:2203.01777 source file (2022-04-21)
Supplement: Supplementary file 3 [file appendix-C.tex]

\begin{figure*}[t]
    \centering
    \includegraphics[width=180mm]{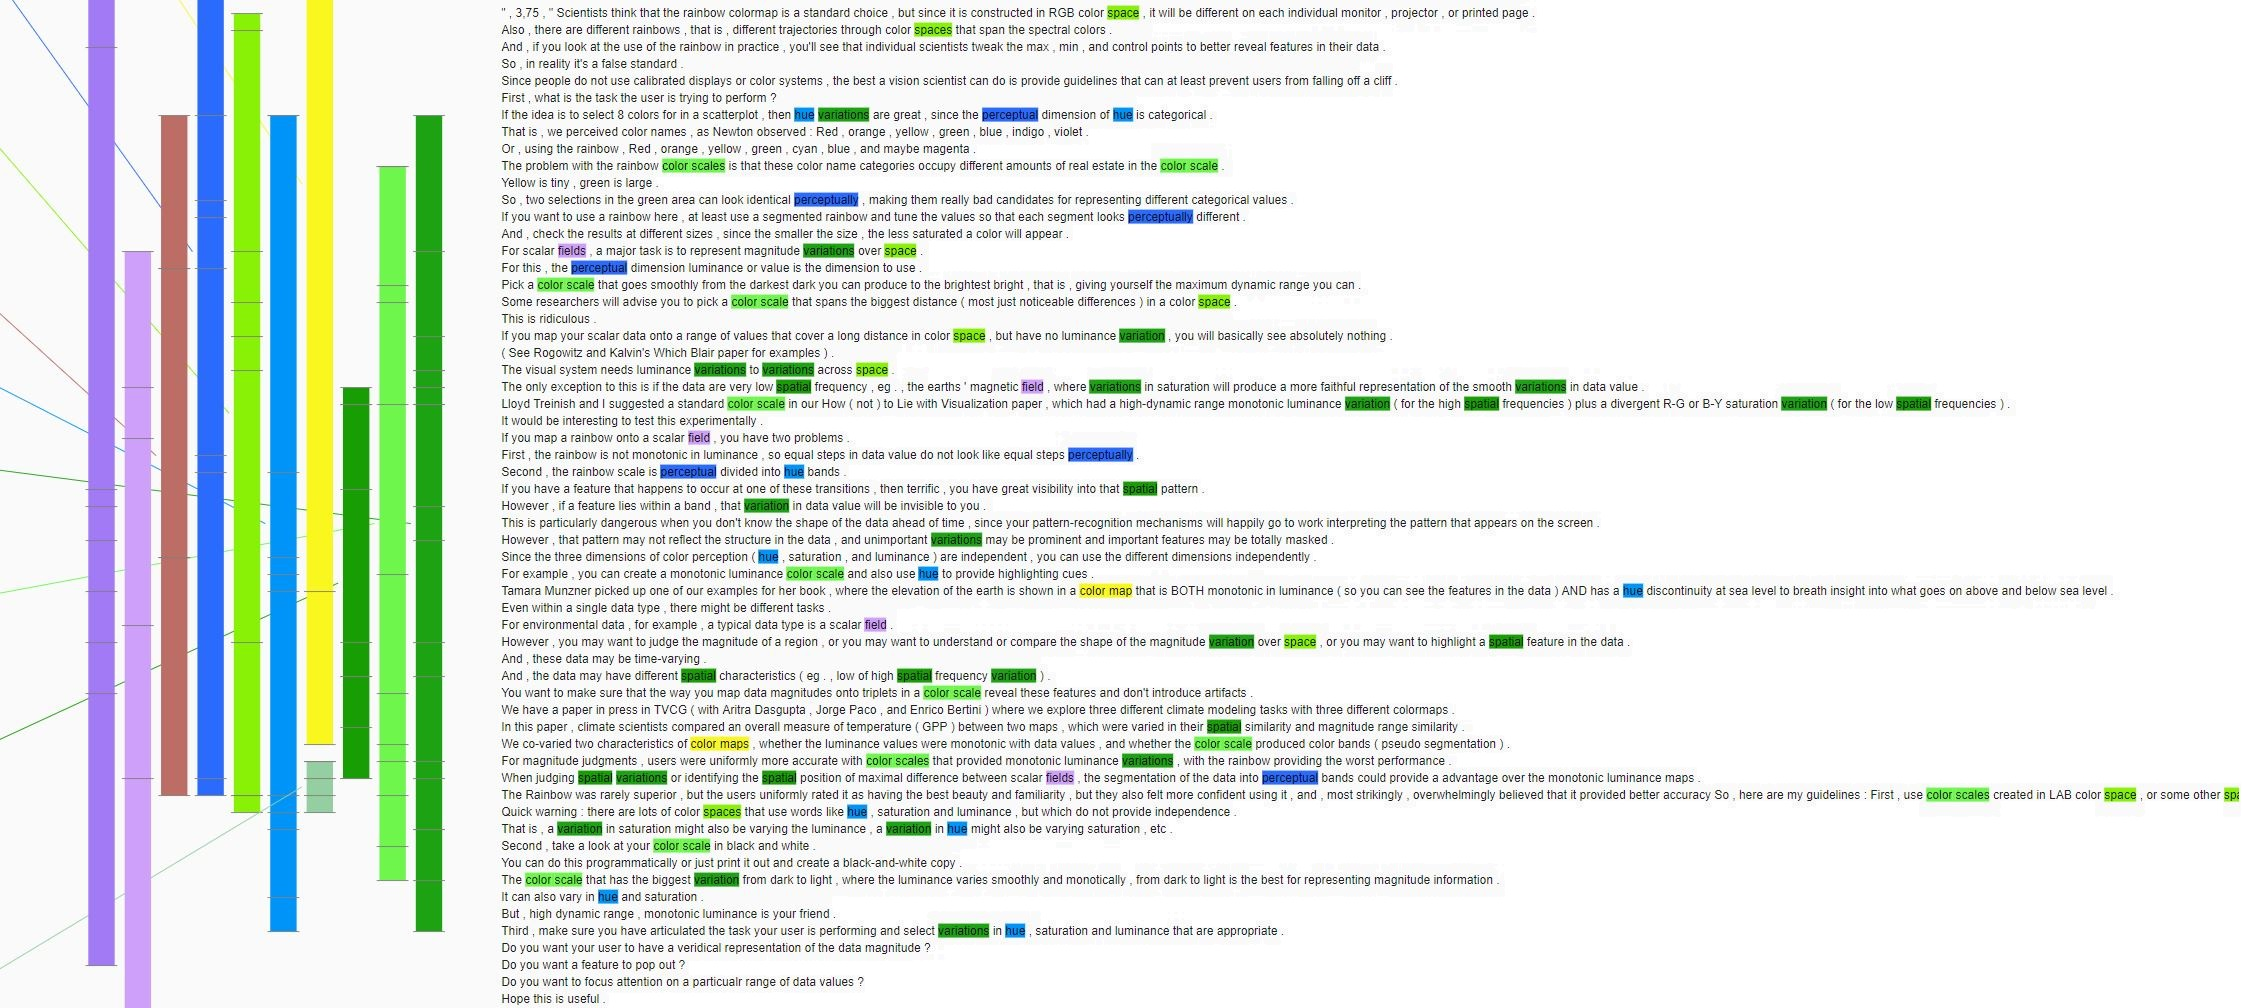}
    \caption{A closely zoomed-in view of a Lexical Episode Plot [30], revealing the interesting text areas for close-reading.}
    \label{fig:LEX-text}
\end{figure*}

\section*{\textbf{C. Further Text Visualization Images}}
\label{app:TextAnalytics}
%
This appendix contains additional visualization images that would br too large for inclusion in Section \ref{sec:TextAnalytics}.

From Fig. \ref{fig:LEP-overview}, we can observe more potential keywords (e.g., \emph{interaction, parallel coordinates, 3D, bubble, etc.} than the zoomed-in view in Fig. \ref{fig:LEP}. Fig. \ref{fig:LEX-text} shows a closely zoomed-in view, enabling users to conduct close-reading of the text that are associated with the identified keywords.

\begin{figure*}[t]
    \centering
    \includegraphics[width=140mm]{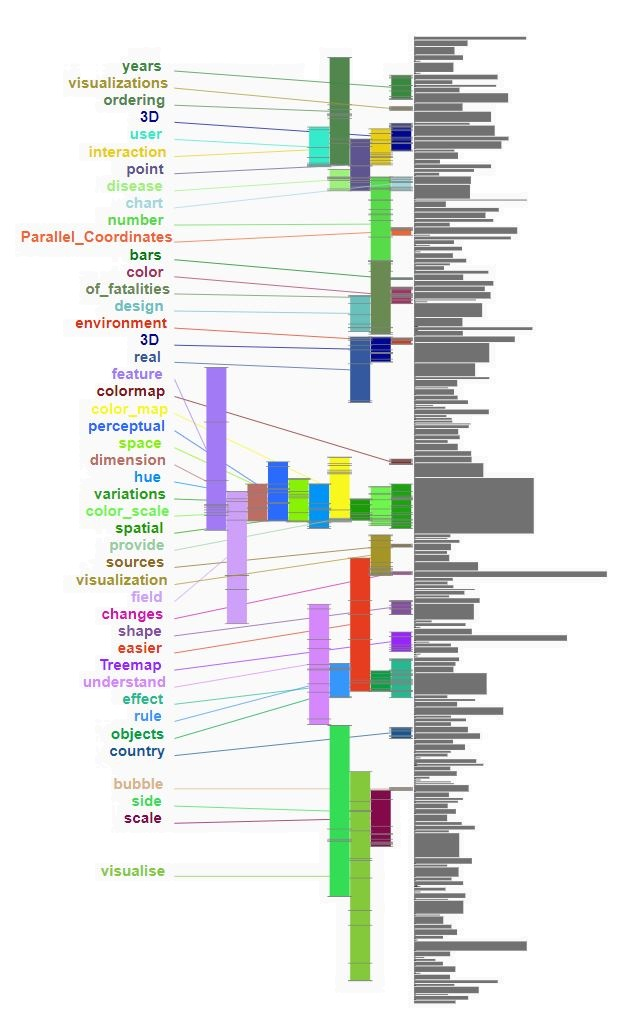}
    \caption{A zoomed-out view of a Lexical Episode Plot [30] showing the evolution of the discussions over time. It automatically detects compact chains of $n$-grams and highlights them beside the complete text as an overview. One can interactively zoom-in to the interesting text areas for close-reading.}
    \label{fig:LEX-overview}
    % \vspace{-20mm}
\end{figure*}

\begin{figure*}[t]
    \centering
    \includegraphics[width=180mm]{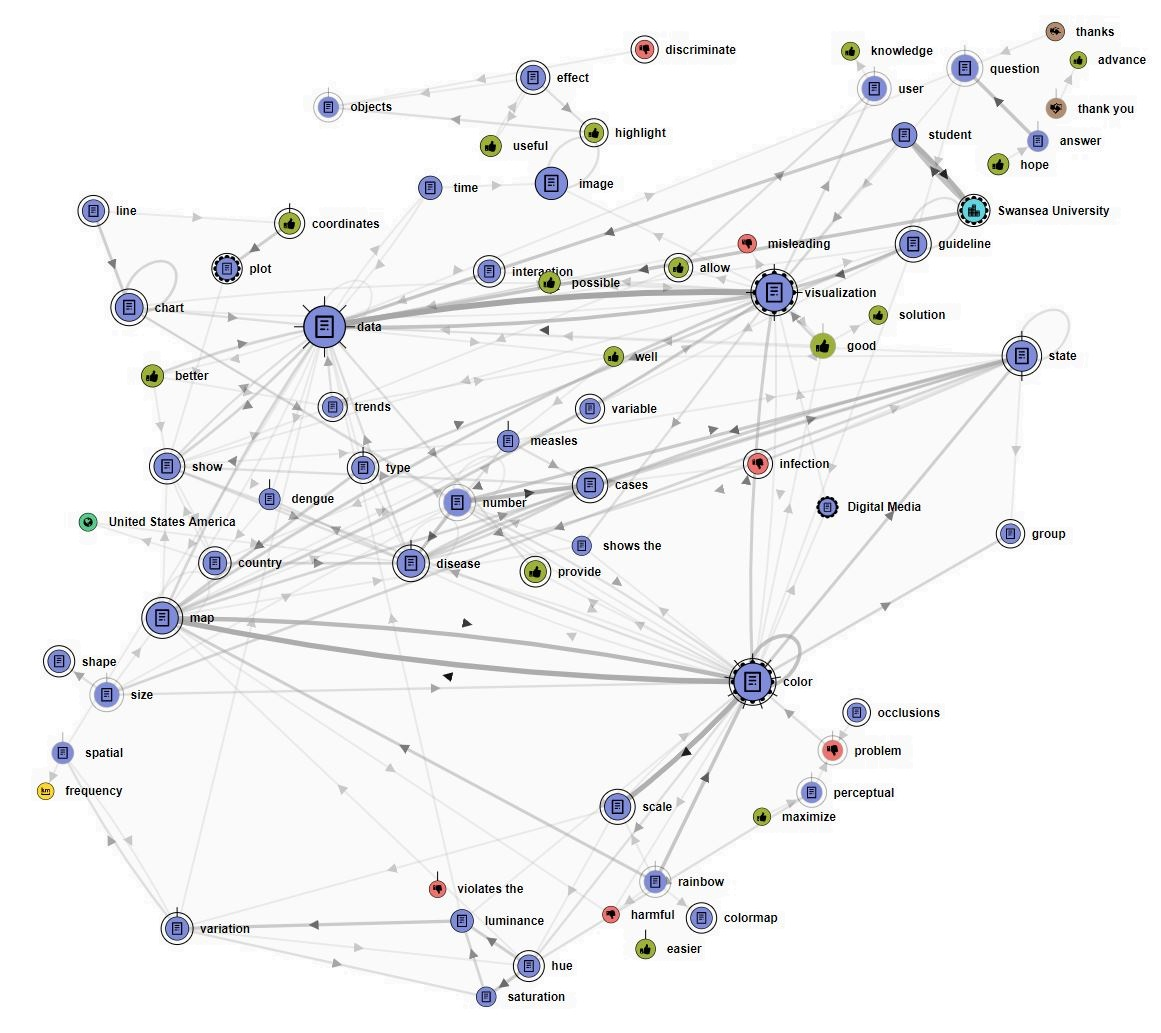}
    \caption{The Named Entity Graph~\cite{El-Assady2017} depicts the relationship between the most \textit{relevant} entity pairs in a corpus, i.e., entities occurring more often together than an expected threshold. In this graph instance,  the node ``color'' is very prominent, as the use of rainbow colormaps has been extensively discussed in the underlying text.}
    \label{fig:NEREx}
\end{figure*}

\begin{figure*}%[hb!]
    \centering
    \includegraphics[width=170mm]{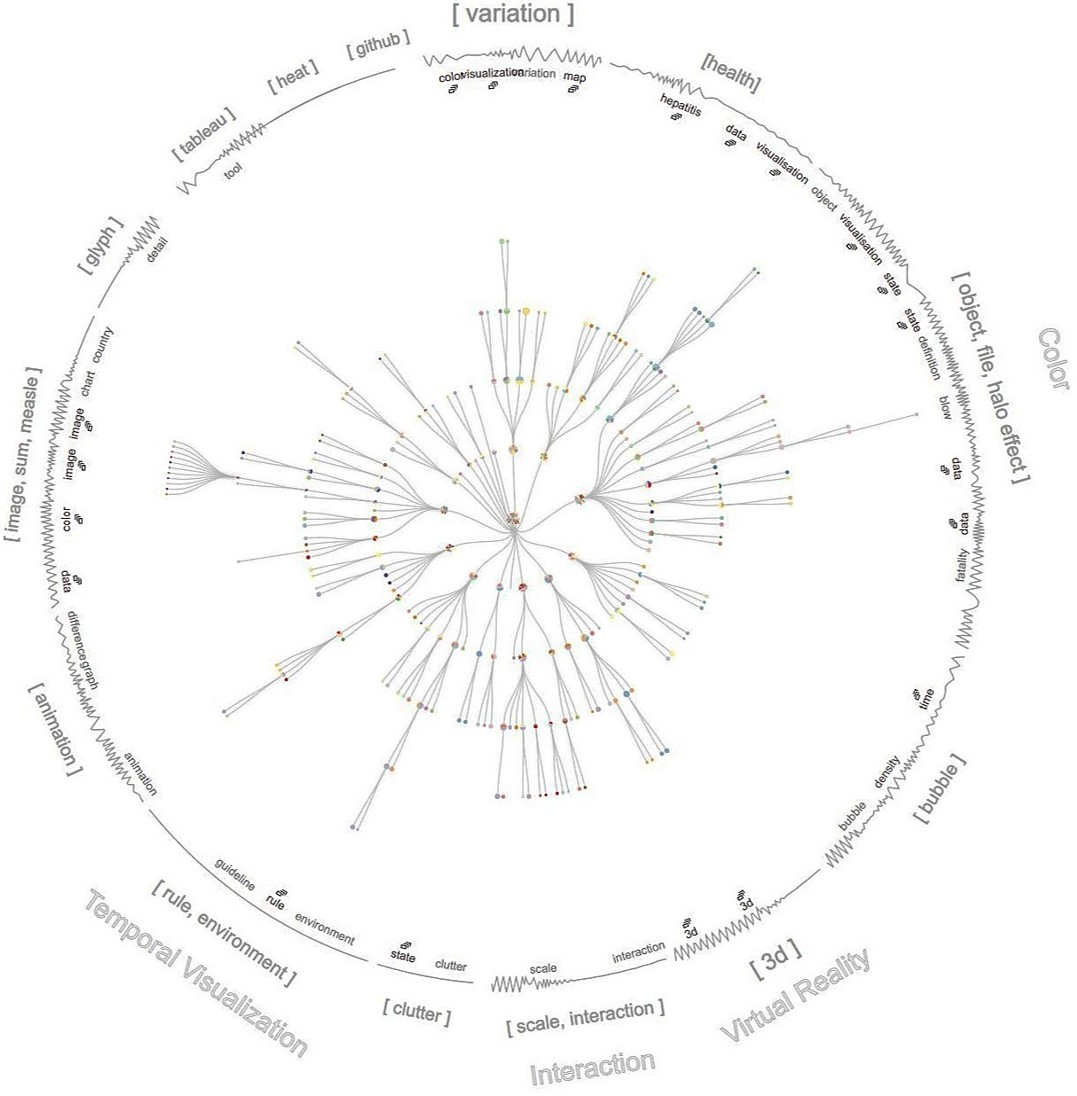}
    \caption{The Topic Tree~\cite{el2018visual} \textit{groups all semantically-related utterances} (as leaf nodes) in a hierarchical tree structure with inner-nodes constituting topics and sub-topics. The \textit{outer border} of the tree depicts the \textit{top-descriptors} of each topic branch and the \textit{uncertainty of the respective utterance assignment} to that topic. }
    \label{fig:topics}
\end{figure*}

\begin{figure*}[t]
    \centering
    \includegraphics[width=180mm, trim={2.3cm 0 1.6cm 0}, clip]{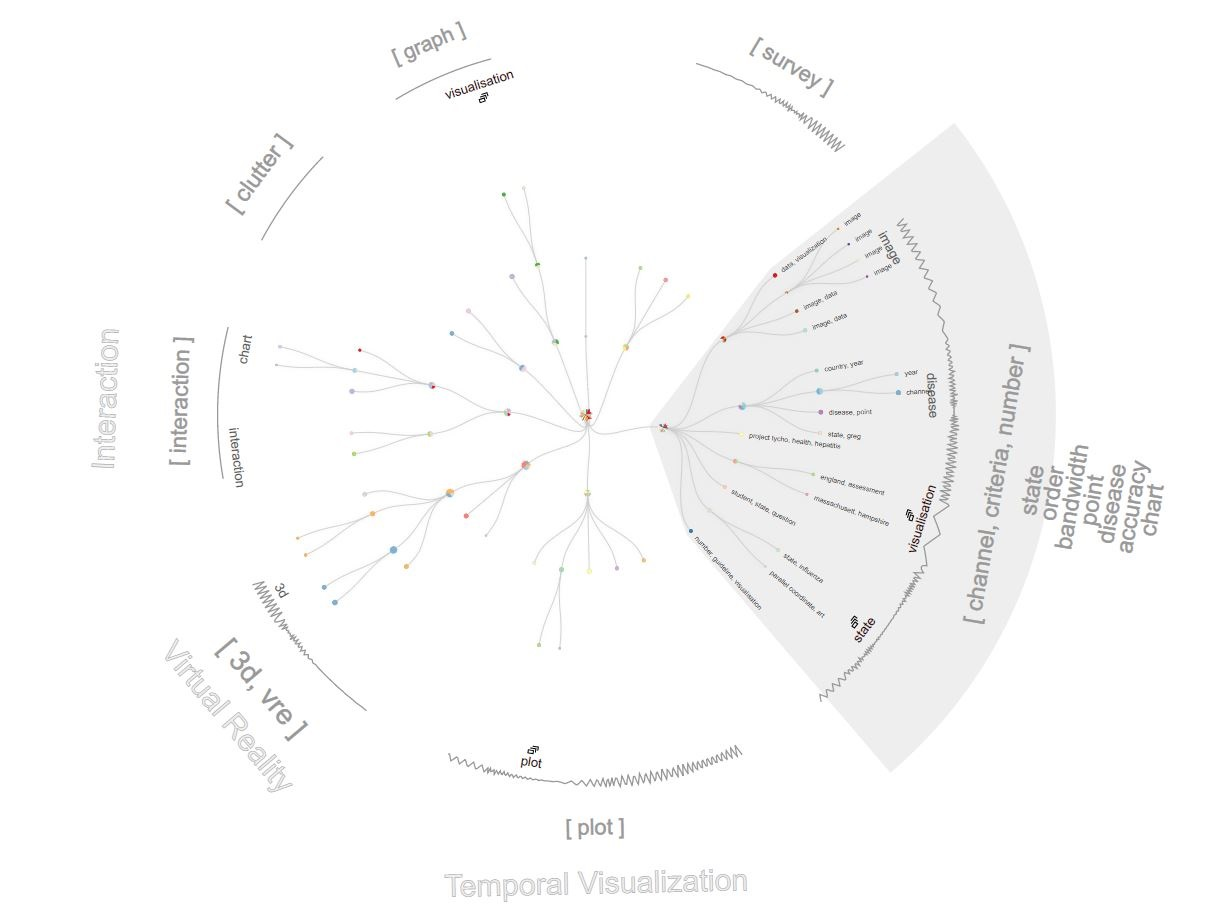}
    \caption{An intermediate result of the  Topic Tree~\cite{el2018visual}, which \textit{groups all semantically-related utterances} (as leaf nodes) in a hierarchical tree structure with inner-nodes constituting topics and sub-topics. The \textit{outer border} of the tree depicts the \textit{top-descriptors} of each topic branch and the \textit{uncertainty of the respective utterance assignment} to that topic. Hovering over a topic segment reveals the top descriptive keywords for that topic.}% (as seen at 3 o'clock).} 
    \label{fig:LEP-overview}
\end{figure*}
