# Supplementary material for: Characterizing Grounded Theory Approaches in Visualization
Source: arXiv:2203.01777 source file (2022-04-21)
Supplement: Supplementary file 4 [file appendix-D.tex]

\section*{\textbf{D. Grounded Theory and VisGuides Data}}
\label{app:OriginalGT}
%
\subsection*{\textbf{D.1 Formal Descriptions of Ground Theory Methods}}
%
\emph{Grounded theory} was proposed in the context of the social sciences \cite{Glaser:1967:book}. Consider a postulated theory $T$ (e.g., about social behaviors), which may be in the form of a categorization scheme, a taxonomy, an ontology, a causal relation, a conceptual model, or a numerical model. The initial theory $T_1$ may be formulated based on a data set $D_1$ (e.g., a collection of news reports on social behaviors). We use $D_1 \hookrightarrow T_1$ to denote the grounded process for deriving $T_1$ from $D_1$.

Grounded theory instigates that the theory $T$ needs to be grounded in the data space $\mathbb{D}$ where $T_1$ emerged, by constantly and continuously sampling the data space, analyzing the data captured, and refining the theory until it reaches theoretical saturation $T_\text{sat}$. In other words, over a long period of time, the sampling collects new data sets $D_2, D_3, \ldots, D_t, \ldots, D_n \in \mathbb{D}$, and the analysis evolves the theory as $T_2, T_3, \ldots, T_t, \ldots, T_\text{sat}$.
%
At each iteration $t$ where a new data set $D_t$ is obtained, grounded theory outlines a number of methods for obtaining $T_t$. As listed in Table \ref{tab:GroundedTheory} that was compiled based on \cite{Willig:2013:book}, these include:
%
\begin{itemize}
    \vspace{-1mm}%
    \item \textbf{Categorization}: deriving a refined theory based on the combined data collection as $\bigcup_{i=1}^t D_i \hookrightarrow T_t$, with aid of other methods below. Here $\bigcup$ denotes the union of data sets.
    \vspace{-1mm}%
    \item \textbf{Coding}: deriving candidates of $T_i$ through close reading of the data set $D_i$. For example, using \emph{open coding}, different people,  $a, b, c, \ldots$, may derive several candidate theories independently:
    \vspace{-1mm}
    \begin{equation*}
      D_i \stackrel{a}{\hookrightarrow} T_{i,a}, \quad
      D_i \stackrel{b}{\hookrightarrow} T_{i,b}, \quad
      D_i \stackrel{c}{\hookrightarrow} T_{i,b}, \quad \ldots   
      \vspace{-1mm}
    \end{equation*}
    %
    \emph{Axial coding} enables the identification of the relationships among the candidate theories, while \emph{selective coding} applies the existing and new candidate theories to different data sets, e.g., $\Xi(T_{i-1}, D_i), \Xi(T_{i,a}, D_{i-1}),$ etc., where we write the application of a theory $T$ using a data set $D$ as a function $\Xi(T, D)$.
    \vspace{-1mm}%
    \item \textbf{Comparative Analysis}: comparing the existing and new candidate theories, for example, by evaluating the applications of these theories to all collected data, $\Xi(T_{i-1}, \bigcup_{i=1}^t D_i), \Xi(T_{i,a}, \bigcup_{i=1}^t D_i),$ etc. or by integrating two or more theories into a new candidate theory and then continuing the comparative analysis. 
    \vspace{-1mm}%
    \item \textbf{Negative Cases Analysis}: identifying negative cases during the coding and comparative analysis, gaining a deep understanding of these cases, and if appropriate, refining the proposed theories.
    \vspace{-1mm}%
    \item \textbf{Memoing}: recording the ideas and actions that lead from the data $D_1, D_2, \ldots, D_i$ to various intermediate theories (e.g., $T_{i,a}, T_{i,b},$ etc.) and eventually to $T_i$.
\end{itemize}

The aforementioned methods embody the three principles of grounded theory, namely:
\begin{itemize}
    \vspace{-1mm}%
    \item \textbf{Theoretical sensitivity}: a theory should be derived from data, validated by data, and remain sensitive to the data \cite{Glaser:2004:FQSR}.
    \vspace{-1mm}%
    \item \textbf{Theoretical sampling}: data collection should be oriented towards the generation, evaluation, and refinement of a theory or theories \cite{Breckenridge:2009:GTR}.
    \vspace{-1mm}%
    \item \textbf{Theoretical saturation}: the process of grounding a theory on data should be constant and continuous until all constructs of a theory are fully represented by the data \cite{Saunders:2018:QQ}.
\end{itemize}

\subsection*{\textbf{D.2 Grounding Visualization Guidelines on Data.}}
%
From the perspective of GT, visualization guidelines are theories that should be grounded on data, since almost all these guidelines were proposed based on the originators' observation and experience, or on the results of empirical studies.

An ideally-formulated visualization guideline $T$ may be expressed as a \emph{construct},  ``doing action $\mathbf{A}$ causes outcome $\mathbf{B}$ under the condition $\mathbf{C}$.''
For example, Correll and Gleicher proposed a guideline: ``in bar charts ($\mathbf{C}$), error bars ($\mathbf{A}$) considered harmful ($\mathbf{B}$)'' \cite{Correll:TVCG:2014}.
Many guidelines are expressed with a construct ``do $\mathbf{A}$'' or ``don't do $\mathbf{A}$.''
The former implies a positive outcome $\mathbf{B}$ (e.g., ``make sure all data adds up to 100\%'' \cite{Kosara:2010:web}), while the latter implies a negative outcome $\mathbf{B}$ (e.g., ``do not use blow-apart effects'' \cite{Duke:2019:web}).

Many guidelines do not explicitly specify any condition $\mathbf{C}$, e.g.,
\begin{center}
\vspace{-2mm}
``Rainbow color map is considered harmful'' \cite{Rogowitz:1998:S,Borland:2007}.\\
``Good visualizations should maximize data-ink ratio'' \cite{tufte2001visual}.\\
``Don't use more than six colours together'' \cite{Sayers:2019:web}.\\
``Pie charts are bad and 3D pie charts are very bad'' \cite{Fenton:2009:web}.   
\end{center}
\vspace{-2mm}
\noindent The omission of $\mathbf{C}$ may suggest the general applicability or a deficit of theoretical sensitivity. There is little doubt that in some conditions $\mathbf{C}_1, \mathbf{C}_2, \ldots$, such guidelines are certainly correct. However, we often do not know what these conditions are, suggesting a need for further theoretical sampling. 

In addition to considering visualization guidelines as individual theories, we can anticipate the possibility of formulating meta-theories that model different aspects of the corpus of visualization guidelines, e.g., their categorization \cite{kandogan2016grounded} and their lifecycle \cite{engelke2018visupply}.
According to grounded theory, such meta-theories should also be grounded on the relevant data, which may include different expressions of the guidelines, the attributes of each expression (e.g., originator, location, period, context, etc.), and documentation about their formulation, discussion, curation, sharing, application, evaluation, refinement, and so on. 

\subsection*{\textbf{D.3 VisGuides: Enabling Grounded Theory Methods}}
%
VisGuides (\url{visguides.org}) is an online discussion forum dedicated to visualization guidelines \cite{Diehl:2018:EuroVis}.
It allows registered users to propose and recommend guidelines, pose questions and offer advice, share positive and negative experience about certain guidelines, report and reason about successes, failures, and conflicts of guidelines, and suggest ways to refine guidelines.
It is a digital platform that features both the ``theories'' (i.e., visualization guidelines) to be developed, and the ``data'' (i.e., discourses) that can be used to generate, evaluate, and refine the theories.
It can support a number of grounded theory methods.

Let $\mathbb{D}_{\text{VisGuides}}$ be the data space of all possible posts at VisGuides. At a point of time $t$, $D_t \in \mathbb{D}_{\text{VisGuides}}$ is the set of posts collected until that time. Hence, VisGuides provides an evolving data set, $D_1 \subseteq D_2, \ldots, D_{t-1} \subseteq D_t$, which is ideal for supporting the principle of theoretical sampling. For a specific context $\Theta$ (e.g., about a datatype, a visual design, a task, an application domain, etc.), one can extract all relevant posts from $D_t$ such that $G$ can be grounded on $D_{t,\Theta} \subset D_t$.
For a specific guideline $G$, this is a special case of context where $\Theta = G$, VisGuides may not have collected sufficient data for grounding $G$ on $D_{t,G}$. A researcher may initiate new discussion about $G$ on VisGuides, or supplement $D_{t,G}$ with data, $E \notin \mathbb{D}_{\text{VisGuides}}$, that is collected outside of VisGuides.

In the following four sections, we will describe a series of research activities that were inspired and guided by the grounded theory methodology. While we employed traditional grounded theory processes, we also utilized our own expertise in computer-assisted data analysis and visualization to complement the traditional processes. These activities are summarized below, where the same tags used in Table \ref{tab:GroundedTheory}, such as $\S_{\ref{sec:VisGuides}} \backsim \S_{\ref{sec:EmpiricalStudies}}$ and $\S_{\text{A}} \backsim \S_{\text{A}}$, relate the GT processes to individual sections and appendices.

\begin{itemize}
    %\vspace{-1mm}%
    \item \textbf{Traditional Categorization and Coding ($\S_{\ref{sec:VisGuides}}$, $\S_{\ref{sec:Teaching}}$, $\S_{\text{A}}$, $\S_{\text{B}}$).} 
   We close-read all 248 posts in the data set $D_{20190313}$, carried out open and axial coding in order to derive categorization schemes as candidate theories. We used selective coding and statistical graphics to evaluate these categorization schemes. We then proposed an integrated categorization scheme that allowed us to obtain several findings.
    %\vspace{-1mm}%
    \item \textbf{Text Analysis and Visualization (Section {\ref{sec:TextAnalytics}}, $\S_{\ref{sec:TextAnalytics}}$, $\S_{\text{C}}$).}
    In conjunction with the traditional approach, we applied several text analysis and text visualization techniques to $D_{20190313}$, which allowed us to observe many patterns that could not be derived from close reading easily.
    %\vspace{-1mm}%
    \item \textbf{Visualization Coursework (Section \ref{sec:Teaching}, $\S_{\ref{sec:Teaching}}$).} With hundreds of guidelines available in the literature \cite{kandogan2016grounded}, it would take a very long time for an individual guideline to receive a good number of hits in sampling. When VisGuides was used to support a piece coursework, we took the opportunity to define a specific context in which the number of applicable guidelines is much smaller and the sampling can be much more intensive. We denote this subset of data as $D_{\text{Swansea2019}} \subset D_{20190313}$. The close-reading and coding of this $D_{\text{Swansea2019}}$ revealed further findings.
    %\vspace{-1mm}%
    \item \textbf{Empirical Studies (Section \ref{sec:EmpiricalStudies}, $\S_{\ref{sec:EmpiricalStudies}}$).}
    When our initial examination on two specific guidelines indicated a lack of data, we followed the GT methodology to collect more data outside VisGuides. We conducted two empirical studies that resulted in two additional data sets $E_{\text{KCL2019}}$ and $E_{\text{Konstanz2019}}$. These data sets provided the two guidelines with supporting evidence.      
\end{itemize}

\clearpage
