# Supplementary material for: Characterizing Grounded Theory Approaches in Visualization
Source: arXiv:2203.01777 source file (2022-04-21)
Supplement: Supplementary file 5 [file appendix-E.tex]

\section*{\textbf{E. Further Details of Empirical Studies}}

\subsection*{\textbf{E.1 A Study Inspired by ``Action without Interaction''}}
%
This section provides further details on the first user study conducted.


% The \emph{apparatus} used for this study includes MS-Excel for Mac (version 16.23) and Tableau Desktop Professional Edition (version 2018.3.3). Both visualization tools were run on macOS High Sierra (version 10.13.6), iMac (Retina 5K, 2017), 3.4 GHz Intel Core i5, 32GB 2400 MHz DDR4, and Radeon Pro 570 4096 MB. Each participant was required to interact with the software using a keyboard and a mouse at the desk. All trials were recorded by both Camtasia and a camera.


\paragraph{\textbf{Design:}}
For each participant, the experiment consisted of four trials, either [\texcel-D1, \ttableau-D2, \ttableau-D3, \texcel-D4] or [\ttableau-D1, \texcel-D2, \texcel-D3, \ttableau-D4]. In each trial, the data set was pre-loaded onto the visualization tools. Participants were given written specification of the tasks together with examples of the bar charts to be created. After an initial attempt of 1 minute for tasks associated with data sets \texttt{D1} and \texttt{D2} and 2 minutes for tasks with data sets \texttt{D3} and \texttt{D4}, participants were allowed to make use of a help-sheet to complete the task. At the end of the second trial, participants ware presented with two questions (for \texttt{T1} and \texttt{T2} with \texttt{D1} and \texttt{D2}) about the easiness of using the two visualization tools. They are asked to rank the relative easiness using the Likert scale. Similarly at the end of the fourth trial, participants were presented with three questions (for \texttt{T1} and \texttt{T2} with \texttt{Ca} and \texttt{Cb}, and for the overall impression).

Because all participants can access a help-sheet with step-by-step instructions for each task (after one minute for \texttt{D1} and \texttt{D2} and two minutes for \texttt{D3} and \texttt{D4}), they were all able to complete the tasks. The accuracy is thus not the focus of this study.

\paragraph{\textbf{Participants.}}
A total of 20 participants (12 females, 8 males) took part in this experiment in return for a \pounds5 Amazon voucher. 
Participants were recruited from King's College London. 
They belong to both the student and working communities and are from a number of disciplines, including history, psychology, business, politics, mathematics, law, and computer science. 
Among them, 17 participants were in the 20-29 age group and 3 were in the 18-19 age group. In rating their experience in using MS-Excel, 3 rated ``beginner'', 16 rated ``intermediate'', and 1 rated ``advanced''. 
In the rating of their experience in using Tableau, 18 rated ``never'', 1 rated ``beginner'', and 1 rated ``intermediate''.

\paragraph{\textbf{Apparatus.}}
The \emph{apparatus} used for this study includes MS-Excel for Mac (version 16.23) and Tableau Desktop Professional Edition (version 2018.3.3). Both visualization tools were run on macOS High Sierra (version 10.13.6), iMac (Retina 5K, 2017), 3.4 GHz Intel Core i5, 32GB 2400 MHz DDR4, and Radeon Pro 570 4096 MB. Each participant was required to interact with the visualization tool using a keyboard and a mouse at the desk as shown in Fig. \ref{fig:KCL-apparatus}. All trials were recorded by both Camtasia and a camera.

% --------------------
\begin{figure}[t]
\includegraphics[width=\columnwidth]{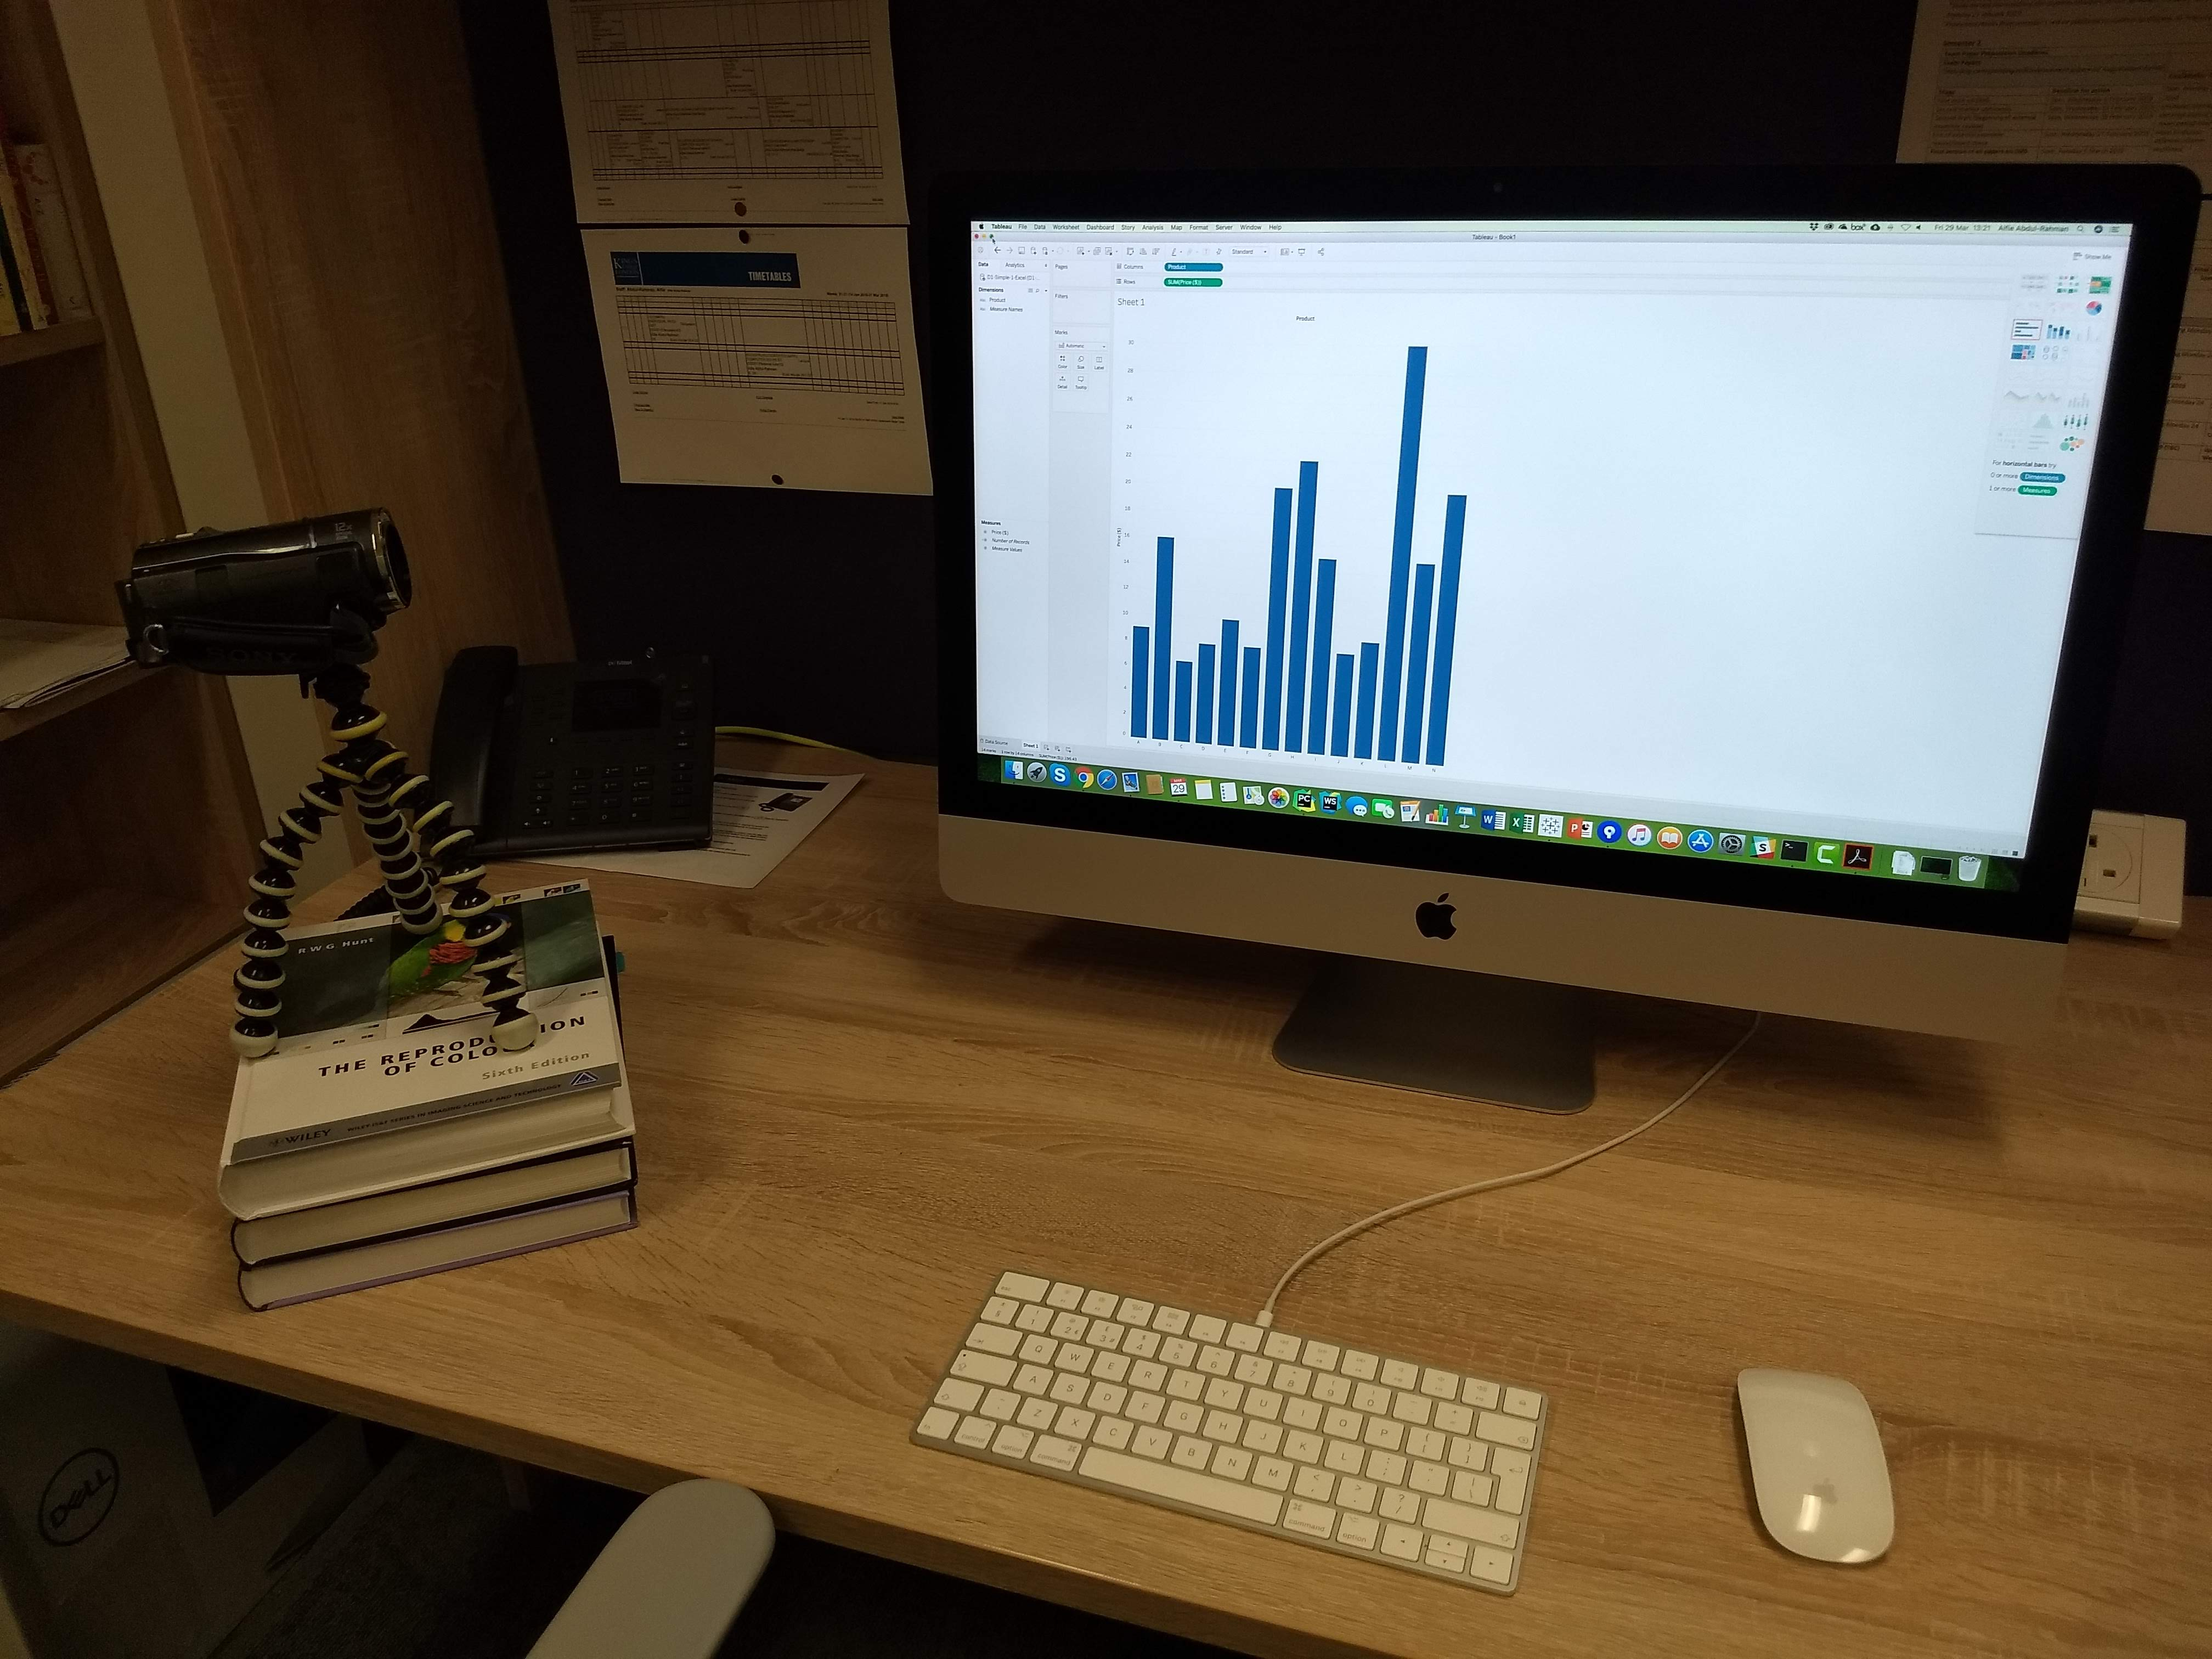}
  \centering
  \caption{Apparatus used in the empirical study on the cost of interaction.}
 \label{fig:KCL-apparatus}
\end{figure}
% --------------------

%\paragraph{\textbf{Procedure.}} We arranged for the participants to take part in the experiment individually. The time taken to complete the experiment was approximately 10-25 minutes, excluding the process for obtaining consent and the pre-study explanation (5 minutes).

Following the protocol of the university an information sheet was first given to the participant during the recruitment process. Before the pre-study explanation, a consent form was distributed for the participant to read and sign. Once the participant has agreed to take part in the study, the experimenter gave a brief explanation to the participant. The explanation included the tasks involved, the access to the help-sheet, and the sequence of the trials. The participants were informed that they could take as much time as they needed in the experiment.
Following the pre-study explanation, each participant was then given a unique anonymous ID, and a demographic form to be completed for information such as gender, age group, occupation, and familiarity with the two visualization tools tested.
%For each participant, the experiment consisted of four trials, either [EXL-Sa, TBL-Sb, TBL-Ca, EXL-Cb] or [TBL-Sa, EXL-Sb, EXL-Ca, TBL-Cb]. In each trial, the data set was pre-loaded onto the visualization tools. Participants were given written specification of the tasks together with examples of the bar charts to be created. After an initial attempt of 1 minute for tasks associated with data sets Sa and Sb and 2 minutes for tasks with data sets Ca and Cb, participants were allowed to make use of a help-sheet to complete the task. At the end of the second trial, participants ware presented with two questions (for T1 and T2 with Sa and Sb) about the easiness of using the two visualization tools. They are asked to rank the relative easiness using the Likert scale. Similarly at the end of the fourth trial, participants were presented with three questions (for T1 and T2 with Ca and Cb, and for the overall impression).





%%%%%%%%%%%%%%%%%

\subsection*{\textbf{E.2 A Study Inspired by ``Don't Replicate the Real World''}}

This section provides further details on the second user study conducted.

\paragraph{\textbf{Data:}}
The data sets used in this study are height fields in the form of $y=H(x,z)$, which are commonly used to depict bi-variate data distributions and terrain landscapes. 
As shown in Fig. \ref{fig:Konstanz-stimuli}, the main data sets in each stimulus are two 
height fields, $D1$ and $D2$, displayed as two 3D surfaces, one floating on the top of another, in a visually-realistic VE. 

\paragraph{\textbf{Task:}} The \emph{visualization task} is to identify the \emph{common peaks} in both surfaces and to select two highest peaks among all common peaks. Here a common peak is defined as the location $(x, z)$ such that $y_1 = H_1(x, z), y_2 = H_2(x, z)$, $y_1 = y_2$, and $(x, y_1, z)$ and $(x, y_2, z)$ are both local maxima. A layer movement required a participant to grab a surface and move it upwards or downwards. When the two surfaces are more separated, one can see the two surfaces more distinctively, and when they are close to each other, one can see the overlapping of the peaks more precisely. 

\paragraph{\textbf{Dependent Variables}} include the task accuracy as the distance from the user selected location to the two highest common peaks ($D_1$, $D_2$), the task completion time ($T$), and the number of layer movements made during each trial ($N_m$). 
As the participants were allowed to take as much time as they wish to complete the task, the task completion time is the main focus of the study. 

\paragraph{\textbf{Setup:}} Participants are randomly divided into two groups. One group began with a block of 15 trials with the plain 3D environment, and then continued with a block of 15 trials with the office-based VE. Another group began with the office-based VE and continued to the plain 3D environment. The stimuli data sets (i.e., the height fields) used in the 30 trials were randomized.

\paragraph{\textbf{Participants:}}
12 participants (2 females, 10 males) were recruited from the Department of Computer Science, University of Konstanz. All had medium to advanced levels of experience in using VR equipment and performing visualization tasks. As each participant completed 15 trials in the plain 3D environment, and 15 trials in the office VE, there are 180 trials in each of the two conditions. 


\paragraph{\textbf{Apparatus.}}
As shown in Fig. \ref{fig:teaser}(c), the main \emph{apparatus} used is a HTC Vive Pro VR headset (GTX1080Ti, SSD, and 16GB RAM). The experiment was carried out in a $7m \times 7m$ physical laboratory, where each participant performed their tasks in the middle of the room while the experimenter sat a few meters away by the computer that controls the virtual environment.
As shown in Fig. \ref{fig:Konstanz-stimuli}, the plain 3D environment contains only a cube on a plane. The top of the cube is the reference plane for the two height fields. The  visually-realistic VE has a $1m^2$ table in the middle of an office environment (walkable area: $5m \times 5m$). The top of the table is the reference plane for the two height fields. 
The virtual office itself is of $7m \times 20m$ including all spaces for the background objects.

%\paragraph{Hypothesis}
% Participants perform worse when a realistic environment is provided. This could be due to distraction and decreased readability of heightmaps for comparison\\

\paragraph{\textbf{Procedure.}}
All participants first attended an introduction session. With aid of presentation slides, we described the concept of height fields and their typical visual representations, such as heat-maps and 3D surfaces (height-maps). Using examples of real world data (e.g., geographical maps with bi-variate distributions of crime rates and arrest rates, participants became accustomed to the visual observation of height fields, the interpretation of peaks and valleys, and the recognition of similar geometric features between two height fields. They were made aware of the tasks to be performed during the experiment, i.e., identifying common peaks.

The participants would then undergo a training session for working with the VR equipment, including interactive controls for navigation and command selection. Each participant was asked to complete 10 interactive tasks, and was required to repeat the exercise until all tasks were completed without errors.

%Participants are randomly divided into two groups. One group began with a block of 15 trials with the plain 3D environment, and then continued with a block of 15 trials with the office-based VE. Another group began with the office-based VE and continued to the plain 3D environment. The stimuli data sets (i.e., the height fields) used in the 30 trials were randomized.
